# Supplementary material for: Large-Scale Image Retrieval with Attentive Deep Local Features
Source: arXiv:1612.06321 source file (2018-02-03)
Supplement: Supplementary file 1 [file appendix.tex]

%!TEX root = ../iccv_main.tex

\section*{A. Dataset Details}
Our dataset contains 1,060,709 images for 12,894 landmarks, which are located at 4,872 cities in 187 countries as illustrated in  \figref{fig:geolocation}.
%
\iffalse
More complete geolocations of the images are illustrated in \figref{fig:geolocation}.
%
\begin{figure}[t]
\begin{center}
   \includegraphics[width=1\linewidth]{figures/DELF_dataset.jpeg}
\end{center}
	\vspace{-15pt}
	\caption{Geolocation distribution of images in our dataset.}
\label{fig:geolocation}
%%\vspace{-10pt}                                                                                                                                                                                                           
\end{figure}
\fi
%
The top-20 countries with most landmarks are shown in \figref{fig:landmark_countries}.
The top-10 cities are London (179), New York (174), Paris (133), Berlin (85), Hong Kong (83), San Francisco (82), Rome (81), Moscow (70), Beijing (68), and Prague (67), where the numbers in parentheses denote the number of landmarks.
There are various kinds of landmarks in our dataset, which include tourist attraction (1969), town (1730), structure (1175), building (898), village (657), museum (451), UNESCO World Heritage Site (368), city (315), and park (278).
Note that we only included landmarks that have at least 3 photos. 
\begin{figure}[h]
\begin{center}
   \includegraphics[width=1\linewidth]{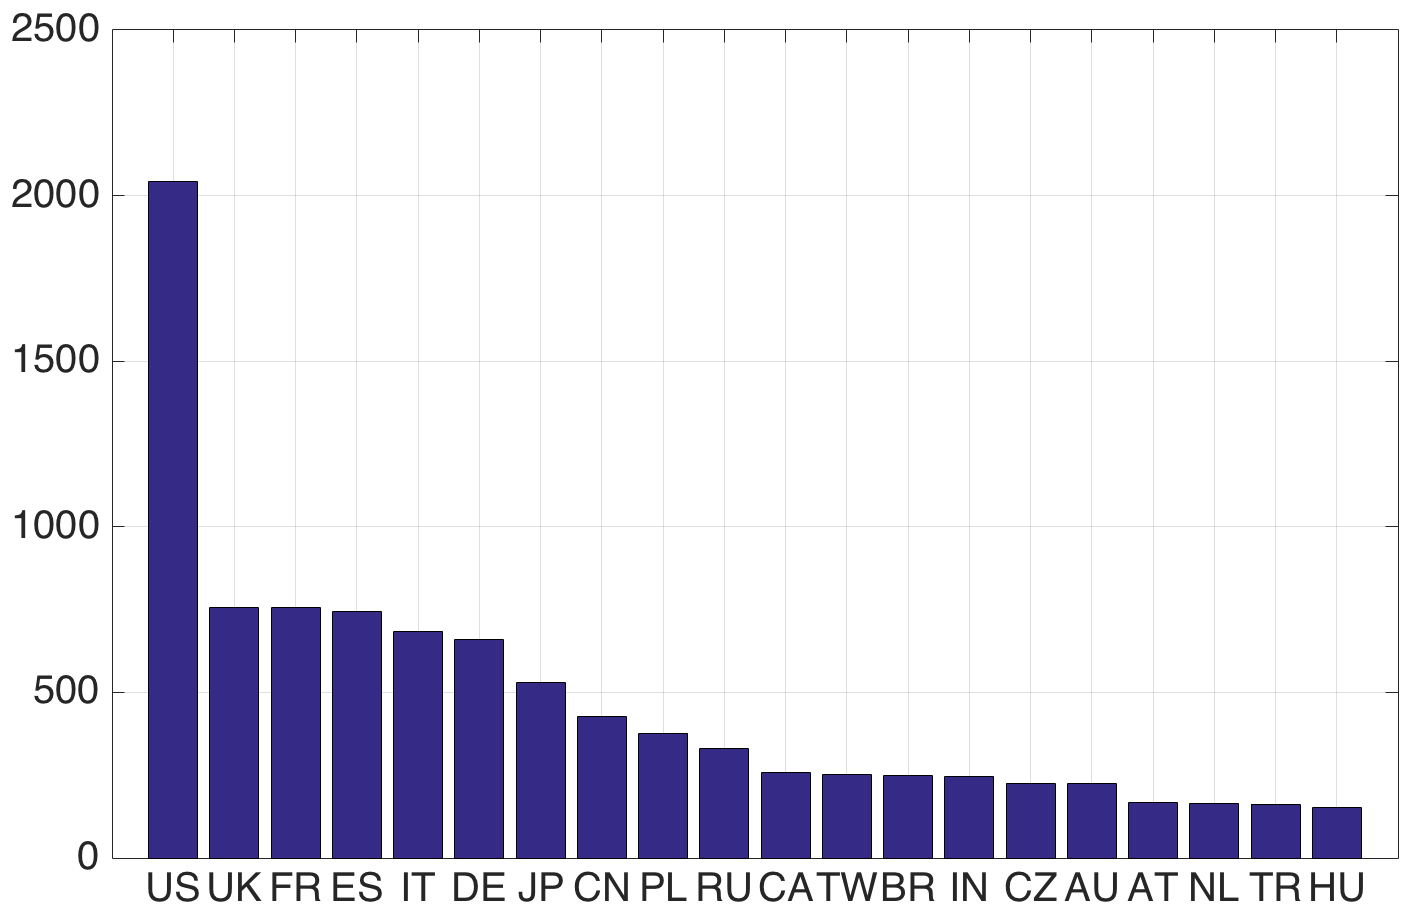}
\end{center}
	\vspace{-15pt}
	\caption{Number of landmarks of top-20 countries in our new dataset.}
\label{fig:landmark_countries}
%\vspace{-10pt}                                                                                                                                                                                                           
\end{figure}
